# Supplementary material for: A kinetic model to simulate charge flow through an electrochemical half cell
Source: arXiv:2507.06197 ancillary file (2025-07-09)
Supplement: Supplementary file 1 [file SI.pdf]

# A kinetic model to simulate charge flow through an electrochemical half cell

Diego Veloza-Diaz,<sup>1</sup> Friederike Schmid,<sup>1</sup> Robinson  
Cortes-Huerto\*,<sup>2</sup> Pietro Ballone,<sup>2</sup> and Nancy C. Forero-Martinez\*<sup>1</sup>

*<sup>1</sup>Institut für Physik, Johannes Gutenberg-Universität Mainz,  
Staudingerweg 9, 55128 Mainz, Germany*

*<sup>2</sup>Max Planck Institute for Polymer Research,  
Ackermannweg 10, 55128, Mainz, Germany*

## I. SELF-DIFFUSION OF IONS IN MC TIME $\tau$

Fig. 1 shows the dependence of the self diffusion coefficient  $D_{MC}$  in MC time as a function of the MC step amplitude  $\Lambda$  and electrolyte concentration  $M$ . The precise definition of  $\Lambda$  is clarified by the following rule for advancing the sample configuration by the attempted MC move from  $\mathbf{r} \equiv (x, y, z)$  to  $\mathbf{r}' \equiv (x', y', z')$ :

$$x' = x + \Lambda \times (\xi_x - 0.5) \quad (1)$$

$$y' = y + \Lambda \times (\xi_y - 0.5) \quad (2)$$

$$z' = z + \Lambda \times (\xi_z - 0.5) \quad (3)$$

where  $\xi_x$ ,  $\xi_y$  and  $\xi_z$  are random numbers extracted from a distribution which is uniform over  $0 < \xi_\alpha < 1$ .

Computations for this SI section have been carried out for cubic samples using the *minimum image convention (mic)* to compute distances among periodic replicas. The attempted moves are accepted with probability  $\nu$  shown in Fig. 2.

The computation of the average square displacement as a function of  $\Lambda$  requires the computation of the average amplitude of a single MC displacement step, i.e.,  $\langle \sqrt{(x - x')^2 + (y - y')^2 + (z - z')^2} \rangle$ .

Deviations of the diffusion coefficient from the quadratic dependence on  $\Lambda$  for interacting particles are due to the rejection of a fraction of the attempted moves, which is measured in Fig. 2 by its complement to 1, i.e., by the acceptance probability. In the case of the non-interacting particles, the acceptance probability of MC moves is identically 1, and  $D_{MC}$  is exactly a quadratic function of  $\Lambda$ , and the fit gives  $a = 0$  and  $b = 8 \cdot 10^{-2}$ . In this case,  $b$  could be determined exactly, but its analytical computation is lengthy because of the cubic pattern of the attempted displacements described by Eqns. 1-3 (instead of the spherical one underlying the elementary treatment of Brownian motion), therefore the quoted value for  $b$  is a numerical estimate.

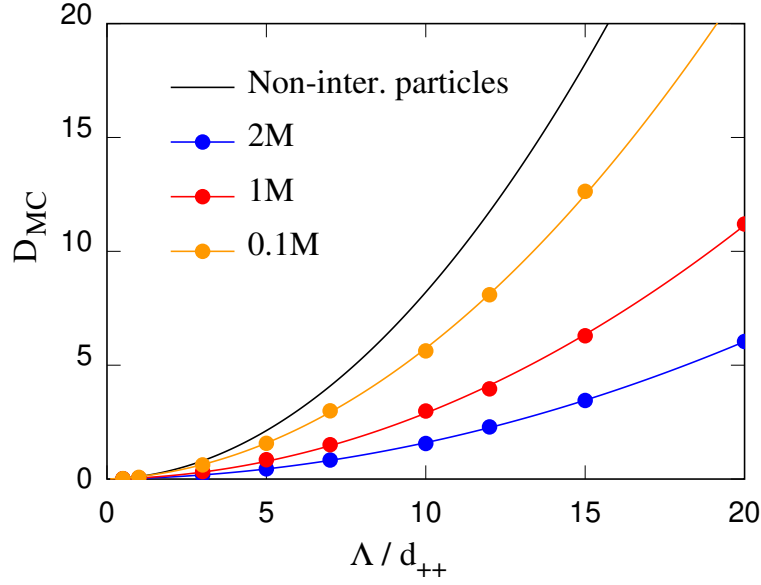

FIG. 1: Self-diffusion constant in MC time as a function of the step  $\Lambda$  for the attempted MC moves. The full lines are quadratic ( $D_{MC} = a\Lambda + b\Lambda^2$ ) interpolations. The curve for non-interacting particles is  $D_{MC} = 0.08\Lambda^2$ .

## II. NOTES ON THE COMPUTATION OF THE ADSORPTION COEFFICIENT AND OF THE CONTACT DENSITY OF CATIONS AND ANIONS IN NEUTRAL ELECTROLYTE SAMPLES

The primary structural property collected during the simulation are the radial profiles  $\rho_+(r)$  and  $\rho_-(r)$  of cations and anions, respectively.

The adsorption coefficient at the interface is defined as:

$$\Gamma_{\pm} = \frac{1}{R_e^2} \int_0^{R_e} r^2 [\rho_{\pm}(r) - \rho_{bulk}] dr \quad (4)$$

and the  $\{\rho_+(R_e), \rho_-(R_e)\}$  density of cations and anions, respectively, at contact:

$$\rho_+(R_e) = \lim_{r \rightarrow R_e} \rho_+(r) \quad (5)$$

with a similar expression for  $\rho_-(R_e)$ .

The computation of  $\Gamma_+$ ,  $\Gamma_-$  is challenging at  $\sigma = 0$  because these are relatively small quantities, heavily affected by equilibrium fluctuations, while the determination of the contact densities is uncertain because these quantities are computed from a histogram of ion numbers

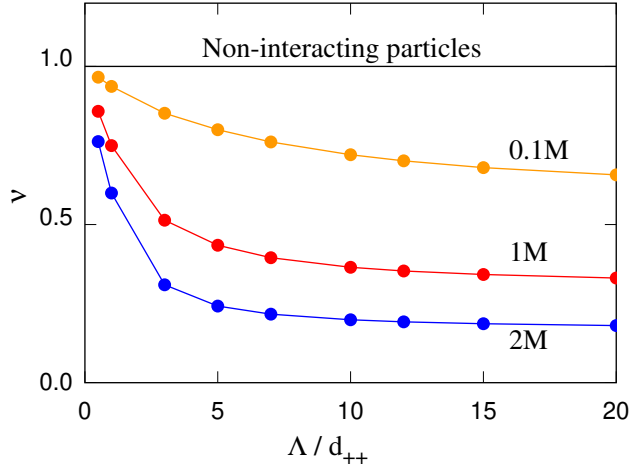

FIG. 2: Acceptance probability of the MC attempted moves of single ions in cubic samples with *minimum image* boundary conditions. The full lines are a guide to the eye. The asymptotic value for large  $\Lambda$  is the probability of inserting one ion at a random position in samples of the given concentration without causing a particle-particle superposition.

on a discrete mesh of radial distances, and the extrapolation to  $r = R_e$  may be affected again by fluctuations but also by systematic errors. To improve their determination, the ionic densities computed on the discrete mesh are first fitted with a constant plus a sum of exponentials centred on the interface and decaying in moving towards the inside of the sample:

$$\rho_\alpha(r) = a_0 + \sum_{i=1}^{n_l} a_i^\alpha \exp \left[ -k_i^{(l)} (R_e - r) \right] \quad i = 1, \dots, n_l \quad (6)$$

where  $\alpha = +, -$ , and  $a_0$  is the bulk density, equal for cations and anions, and of course  $k_i^{(l)}$  is an inverse length.

The  $\{k_i^{(l)}\}$  form a relatively short arithmetic sequence, whose length and spacing among successive elements depends on the molar concentration. For instance, for the 2M case (rapid screening of the interface), 18 exponential basis functions have been used, from  $k_1^{(l)}/d_{++} = 1$  to  $k_{18}^{(l)}/d_{++} = 4.4$  with spacing  $\delta/k^{(l)}d_{++} = 0.2$ . In the 0.1M case (slow screening of the interface,

14 exponential functions have been used, again with  $\delta k^{(l)}/d_{++} = 0.2$ , spanning the interval from  $k_1^{(l)}/d_{++} = 0.3$  to  $k_{14}^{(l)}/d_{++} = 2.9$ . The number of basis functions has been optimised for accuracy but also for stability of the fit.

The fit is very accurate, limited only by the fluctuations of the simulation data. Once the fit has been carried out, the  $\Gamma_\alpha$  and the  $\rho_\alpha(R_e)$  are computed as:

$$\Gamma_\alpha = \sum_{i=1}^{n_l} a_i^\alpha \frac{\int_{r=0}^{R_e} R_e r^2 \exp \left[ -k_i^{(l)} (R_e - r) \right] dr}{R_e^2} = \sum_{i=1}^{n_l} \frac{a_i^\alpha}{k_i^{(l)}} \left[ 1 - \exp \left( -k_i^{(l)} R_e \right) \right] \quad (7)$$

$$\rho_\alpha(R_e) = a_0 + \sum_{i=1}^{n_l} a_i^\alpha \quad (8)$$

### III. ELECTROSTATIC POTENTIAL DROP AT THE INTERFACE, SCREENING LENGTH AND INTERFACIAL CAPACITANCE

The electrostatic potential drop  $\Delta\phi$  measured from the interface to the centre of the spherical sample has been computed as a function of the surface charge density  $\sigma$  for systems of nominal 8000 ions, using Eq. 18 of the main text. The results are collected in Fig. 3.

Given the well known propensity for hyperbolic functions of simple theories (Poisson-Boltzmann type) of the electrostatic double layer, a fit of the data has been attempted with the two-parameters form:

$$\Delta\phi = \alpha \sinh^{-1} [\sigma/\beta] \quad (9)$$

in which  $\alpha$  and  $\beta$  need to be optimised for every value of the electrolyte solution concentration. In practice,  $\alpha$  represents an overall amplitude scale for the potential drop over the diffuse part of the interfacial double layer, and  $\beta$  determines highest curvature of the  $\Delta\phi(\sigma)$  function.

As apparent from the data shown in Fig. 3, the fit is very accurate and gives us an opportunity to compute the differential capacitance  $C_D$  of the samples over the entire range explored by the simulation. The differential capacitance per unit area of the spherical interface satisfies the relation:

$$C_D^{-1} = \frac{\partial \Delta\phi}{\partial \sigma} \quad (10)$$

Considering the analytical form of the fit, the differential capacitance can be computed as:

$$C_D = \frac{\beta}{\alpha} \sqrt{1 + \left( \frac{\sigma}{\beta} \right)^2} \quad (11)$$

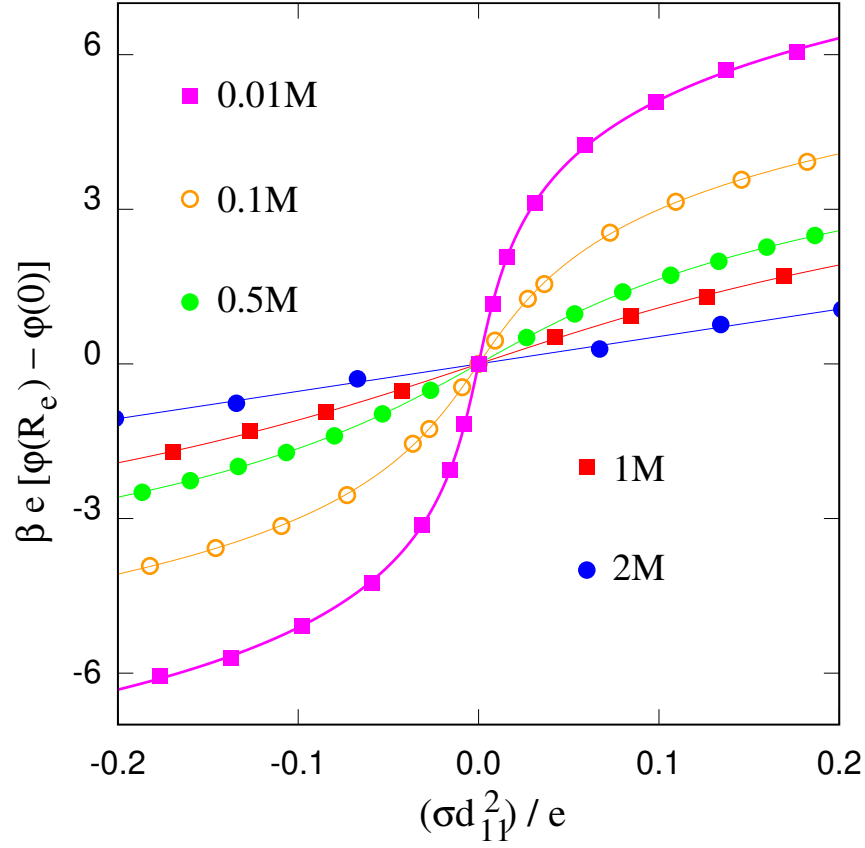

FIG. 3: Electrostatic potential drop across the electrified interface as a function of the surface charge density  $\sigma$ .  $\beta = 1/k_B T$ ,  $\varphi(R_e)$  and  $\varphi(0)$  are the electrostatic potential at the interface and at the centre of the spherical sample, respectively.

The results are shown in Fig. 4

The inverse  $C_D^{-1}$  of the differential capacitance is a measure of the thickness of the diffuse part of the double layer at electrified interfaces. Therefore, it is also a measure of the screening of electrostatic charge at the interface. For this reason,  $C_D^{-1}(\sigma)$  has been reported in Fig. 5, showing that the screening length becomes progressively longer with decreasing concentration. With increasing surface charge, however, even low concentration electrolyte solution accumulate sufficient charge at the interface to be able to effectively screen any electrostatic charge over a

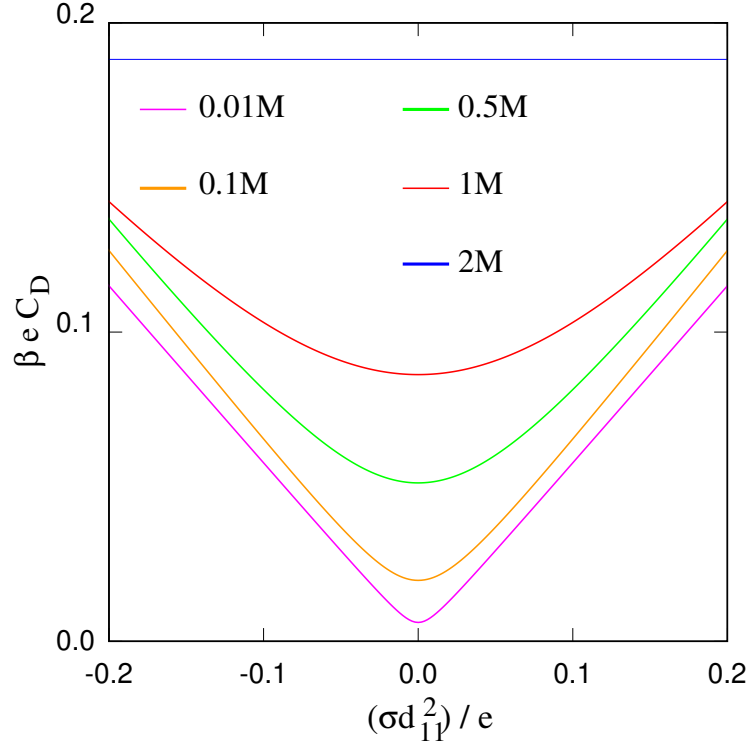

FIG. 4: Differential capacitance  $C_D$  per unit area of the electrode/electrolyte interface as a function of the surface charge for all the electrolyte concentrations considered in the present study.

length that rapidly decreases with increasing  $|\sigma|$ .

#### IV. VERIFICATION OF THE CONTACT DENSITY RELATION FOR ELECTROLYTE IONS AS A FUNCTION OF THE SURFACE CHARGE DENSITY $\sigma$

For neutral interfaces ( $\sigma = 0$ ), the adsorption of the electrolyte on the metal electrode turns from slightly non-wetting to slightly wetting with increasing density (see Tab. I).

The results for neutral systems have been extended to charged surfaces (see Fig. 7).

The contact density relation is derived for a planar interface in Ref. 29 of the main text, and applied without correction to the spherical interfaces of the present study.

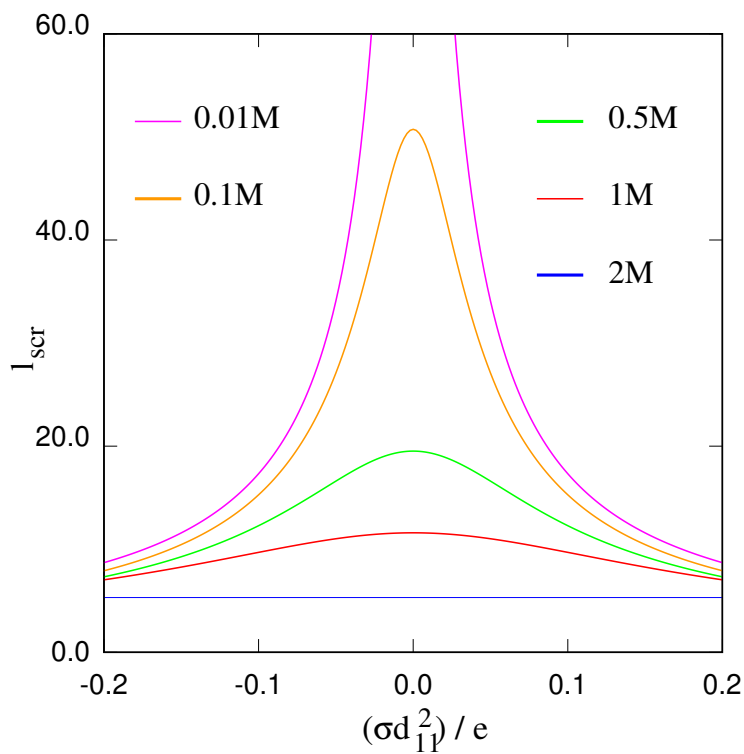

FIG. 5: Screening length of charge imbalance at the electrode/electrolyte interface, measured by the inverse differential capacitance  $l_{scr}(\sigma) = C_D^{-1}(\sigma)$ .

TABLE I: Excess osmotic pressure  $\beta P/\rho - 1$

| Concentration      | 2M          | 1M          | 0.5M                | 0.1M                | 0.01M               |
|--------------------|-------------|-------------|---------------------|---------------------|---------------------|
| $\beta P/\rho - 1$ | $0.349 \pm$ | $0.100 \pm$ | $-(4.4 \pm)10^{-3}$ | $-(5.4 \pm)10^{-2}$ | $-(2.5 \pm)10^{-2}$ |

## V. AVERAGE DENSITY OF ACTIVE ION AS A FUNCTION OF SURFACE CHARGE DENSITY AND ELECTROLYTE CONCENTRATION

Each point of the curves in Fig. 7 is close to the corresponding point in Fig. 6 of the main text, once it is multiplied by  $k_e$ . In other terms,  $j(r)$  is nearly equal to  $k_e \times \langle n_A \rangle$ . This is partly

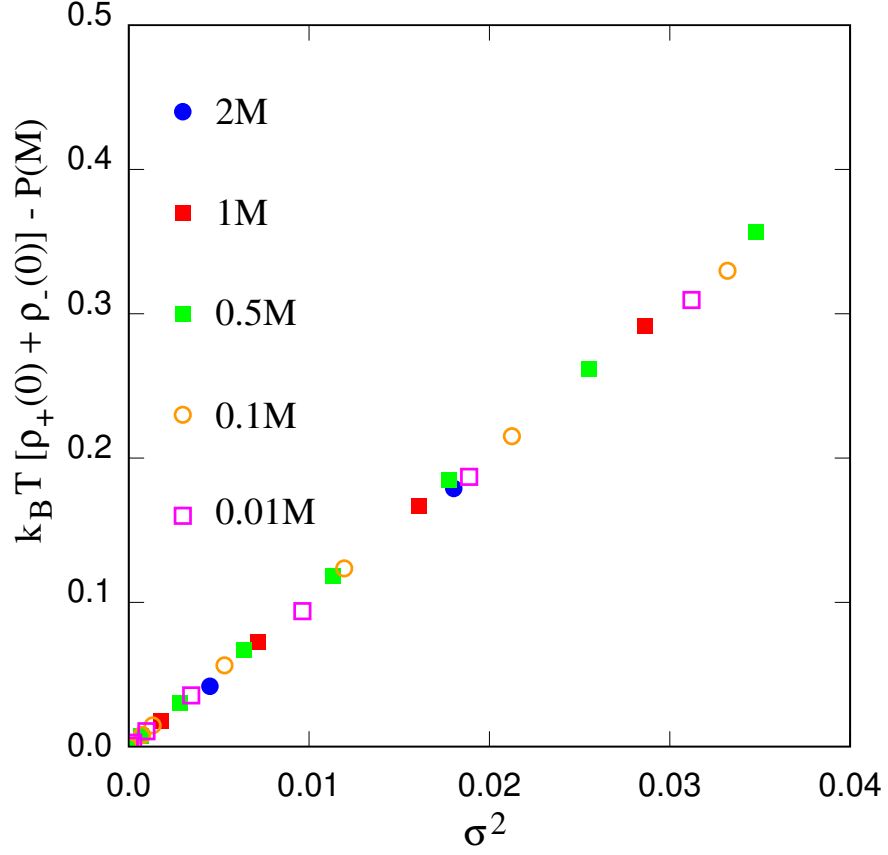

FIG. 6: Contact density of electrolyte ions as a function of concentration, minus the pressure  $P(M)$  of the ions in the bulk-like region of the simulated samples. The contact theorem of Ref. 29 (main text) implies that this quantity depends quadratically on the surface charge density.

due to the simplicity of the simulated model, that neglects the dependence of the transfer rate on the value and fluctuations of the electrostatic potential at the interface.

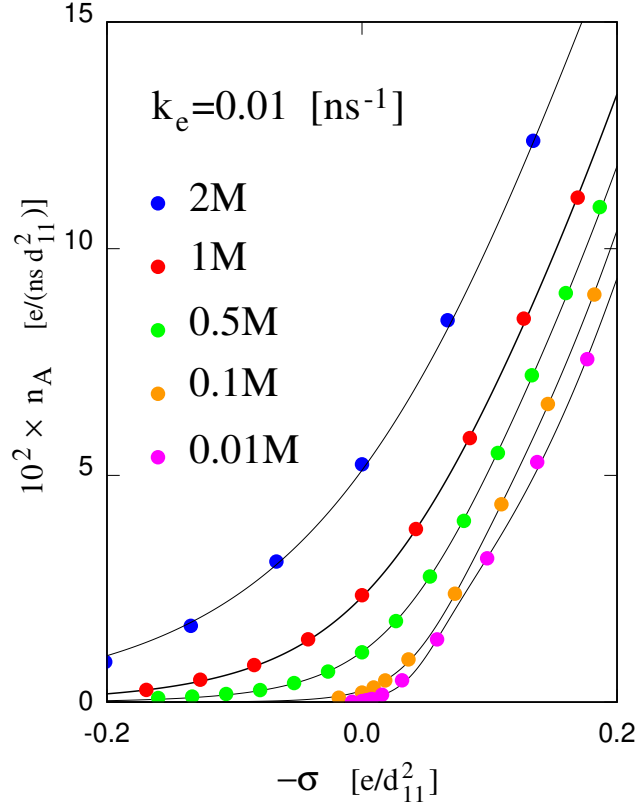

FIG. 7: Average density of active ions as a function of surface charge density  $\sigma$  and electrolyte concentration  $M$ .

## VI. SIZE DEPENDENCE OF THE CURRENT DENSITY $j_r$ AT CONSTANT SURFACE CHARGE DENSITY

To assess the dependence of the simulation results on the curvature of the interface, Tab. II reports the computed radial current density as a function of a few (relatively low) surface charge densities for all the system sizes considered in the present study. It is apparent that the size dependence of the computed  $j_r(R_e)$  is low.

TABLE II: Radial current density at the interface  $j_r(R_e)$  in units of  $10^{-4} \text{ e}/(\text{d}_{++}^2 \text{ ns})$  as a function of surface charge density  $\sigma$ .

| Concentr.         | 2M                                    | 1M              | 0.5M            | 0.1M              | 0.01M              |
|-------------------|---------------------------------------|-----------------|-----------------|-------------------|--------------------|
| $\sigma d_{++}^2$ | 0.1067                                | 0.06723         | 0.04235         | 0.01441           | 0.00312            |
| N                 | $10^4 j_r(d_{11}^2/e) \text{ per ns}$ |                 |                 |                   |                    |
| 4000              | $10.8 \pm 0.4$                        | $5.06 \pm 0.06$ | $2.38 \pm 0.05$ | $0.408 \pm 0.007$ | $0.0342 \pm 0.002$ |
| 8000              | $10.4 \pm 0.4$                        | $5.00 \pm 0.06$ | $2.38 \pm 0.04$ | $0.399 \pm 0.008$ | $0.0345 \pm 0.002$ |
| 16000             | $10.5 \pm 0.3$                        | $4.89 \pm 0.08$ | $2.39 \pm 0.05$ | $0.408 \pm 0.008$ | $0.0357 \pm 0.001$ |
